# Supplementary material for: MERaLiON-AudioLLM: Bridging Audio and Language with Large Language Models
Source: arXiv:2412.09818 source file (2025-01-16)
Supplement: Supplementary file 1 [file appendix.tex]

\section{Statistics of datasets}
\begin{table}[ht!]
    \centering
    \begin{tabular}{cccc}
    \toprule
    \textbf{Dataset} & \textbf{Train} & \textbf{Dev} & \textbf{Test} \\ 
    \midrule
     \emph{National Speech Corpus} &  & &  \\   
     \cmidrule[0.1pt]{1-1}
      Part 1 & 3350 & - & 7.44 \\ 
      Part 2 & 3150 & - & 6.34 \\  
      Part 3 & 901.32 & - & 31.5 \\  
      Part 4 & 966.87 & - & 30.82 \\  
      Part 5 & 1554 & - & 55.96 \\  
      Part 6 & 1319 & - & 36.72\\  
      \midrule
     \emph{LibriSpeech} & 961.04† & - & 10.74 \\          
     \emph{GigaSpeech} & 9997.82 & 12 & 40 \\         
     \emph{People's Speech} & 5894.75 & 33 & 60 \\ 
     \emph{Common Voice 17 - En} & 1688.78 & 27.31 & 18.17 \\ 

    \bottomrule
    \end{tabular}
    \caption{Automatic Speech Recognition (ASR) datasets} 
    \label{tab:asr_stats}
\end{table}

\begin{table}[ht!]
    \centering
    \begin{tabular}{cccc}
    \toprule
    \textbf{Dataset} & \textbf{Train} & \textbf{Dev} & \textbf{Test} \\ 
    \midrule

     \emph{CoVoST-2} &  &  &  \\     
     \cmidrule{1-1}
     En $\rightarrow$ Zh & 364.44 & 26.10 & 24.65 \\
     En $\rightarrow$ Id & 364.44 & 26.10 & 24.65 \\
     En $\rightarrow$ Ta & 364.44 & 26.10 & 24.65 \\

     Zh $\rightarrow$ En & 10.44 & 7.90 & 8.24 \\
     Id $\rightarrow$ En & 1.21 & 0.86 & 0.91 \\
     Ta $\rightarrow$ En & 1.51 & 0.45 & 0.99 \\
     \midrule
    \emph{GigaSpeech} &  &  &  \\     
     \cmidrule{1-1}
     En $\rightarrow$ Zh & 8559.22 & - & 33.88 \\
     En $\rightarrow$ Ms & 8559.22 & - & 33.88 \\
     \midrule
    \emph{People's Speech} &  &  &  \\     
     \cmidrule{1-1}
     En $\rightarrow$ Zh & 5894.74 & - & 59.80 \\
     En $\rightarrow$ Ms & 5894.74 & - & 59.80 \\
     \midrule
         
    \emph{Common Voice 17} &  &  &  \\     
     \cmidrule{1-1}
     En $\rightarrow$ Zh & 1738.50 & - & 26.96 \\
     En $\rightarrow$ Ms & 1738.50 & - & 26.96 \\
    \bottomrule
    \end{tabular}
    \caption{Speech Translation (ST) datasets}
    \label{tab:st_stats}
\end{table}

\begin{table*}[htb]
    \centering
    \begin{tabular}{cccc}
    \toprule
    \textbf{Dataset} & \textbf{Train} & \textbf{Dev} & \textbf{Test} \\ 
    \midrule

    SLUE-SQA-5 & 511.24 & - & 26.31 \\

    Dream & 57.36 & - & 18.14 \\
    ODSQA & - & - & 41.70 \\
    CN College Entrance English Test & - & - & 13.30 \\
    \midrule
    \emph{Synthesized SQA datasets} &  &  &  \\     
     \cmidrule{1-1}
    Spoken SQuAD & 611.55 & - & 90.74 \\
    NSC Part 3 & 939.96 & - & 33.18 \\
    NSC Part 4 & 895.20 & - & 28.19 \\
    NSC Part 5 & 899.85 & - & 31.01 \\
    NSC Part 6 & 946.19 & - & 26.53 \\
    Common Voice 17 SQA & 1360.08 & - & 18.17 \\
    GigaSpeech SQA & 8464.07 & - & 33.69 \\
    People's Speech SQA & 5865.74 & - & 54.09 \\
    \emph{LibriSpeech SQA} & 959.87 & - & 10.7  \\ 
    Singapore Public Speech SQA & - & - & 7.62 \\

    \bottomrule
    \end{tabular}
    \caption{Spoken Question Answering (SQA) datasets} 
    \label{tab:sqa_stats}
\end{table*}

\begin{table}[htb]
    \centering
    \begin{tabular}{cccc}
    \toprule
    \textbf{Dataset} & \textbf{Train} & \textbf{Dev} & \textbf{Test} \\ 
    \midrule

     \emph{National Speech Corpus} &  &  &  \\     
     \cmidrule{1-1}
        PART 3 & 941.85 & - & 33.23 \\
        PART 4 & 896.86 & - & 28.27 \\
        PART 5 & 901.10 & - & 31.10 \\
        PART 6 & 947.18 & - & 26.54 \\

    \bottomrule
    \end{tabular}
    \caption{Spoken Dialogue Summarization (SDS) datasets}
    \label{tab:sds_stats}
\end{table}

\begin{table}[htb]
    \centering
    \begin{tabular}{cccc}
    \toprule
    \textbf{Dataset} & \textbf{Train} & \textbf{Dev} & \textbf{Test} \\ 
    \midrule

    Alpaca-GPT4-TTS & 37.60 & - & 2.58 \\
    Open Hermes-TTs & 1186.18 & - & 9.97 \\

    \bottomrule
    \end{tabular}
    \caption{Speech Instruction (SI) datasets}
    \label{tab:si_stats}
\end{table}

\begin{table}[htb]
    \centering
    \begin{tabular}{cccc}
    \toprule
    \textbf{Dataset} & \textbf{Train} & \textbf{Dev} & \textbf{Test} \\ 
    \midrule

     \emph{National Speech Corpus} &  &  &  \\     
     \cmidrule{1-1}

    \underline{\textbf{Part 3}} & & & \\
    GR & 4128.77 & - & 138.79 \\
    NR & 3839.15 & - & 129.71 \\
    MIX & 4439.39 & - & 149.41 \\

    \underline{\textbf{Part 4}} & & & \\
    GR & 3988.82 & - & 122.22 \\
    NR & 3713.94 & - & 114.44 \\
    MIX & 4286.47 & - & 130.94 \\

    \underline{\textbf{Part 5}} & & & \\
    GR & 4001.46 & - & 138.27 \\
    NR & 3735.38 & - & 128.31 \\
    MIX & 4326.97 & - & 148.48 \\
    \midrule

    \emph{MELD} &  &  &  \\     
    \cmidrule{1-1}
     
    ER & 8.72 & - & 2.43 \\
    SR & 8.72 & - & 2.43 \\
    \midrule
    \emph{VoxCeleb1} &  &  &  \\     
    \cmidrule{1-1}
    GR & 340.40 & - & 11.20 \\
    NR & 340.40 & - & 11.20 \\

    \bottomrule
    \end{tabular}
    \caption{Statistics of our Paralinguistics (PARA) datasets} 
    \label{tab:para_stats}
\end{table}

\begin{table}[ht!]
    \centering
    \begin{tabular}{cccc}
    \toprule
    \textbf{Dataset} & \textbf{Train} & \textbf{Dev} & \textbf{Test} \\ 
    \midrule

    AudioCaps & 123.46 & - & 12.05 \\
    WavCaps & 785.90 & - & 4.92 \\

    \bottomrule
    \end{tabular}
    \caption{Statistics of our Audio Captioning datasets}
    \label{tab:ac_stats}
\end{table}

\begin{table}[ht!]
    \centering
    \begin{tabular}{cccc}
    \toprule
    \textbf{Dataset} & \textbf{Train} & \textbf{Dev} & \textbf{Test} \\ 
    \midrule

    AudioCaps ASQA & 121.77 & - & 11.89 \\
    WavCaps ASQA & 766.43 & - & 4.84 \\
    Clotho ASQA & 35.26 & - & 14.12 \\

    \bottomrule
    \end{tabular}
    \caption{Statistics of our Audio Scene Question Answering (ASQA) datasets}
    \label{tab:asqa_stats}
\end{table}
